# Supplementary material for: Ergodicity Breaking and High-Dimensional Chaos in Random Recurrent Networks
Source: arXiv:2510.07932 source file (2025-10-09)
Supplement: Supplementary file 1 [file SM.pdf]

# Supplemental Material: Ergodicity Breaking and High-Dimensional Chaos in Random Recurrent Networks

**Carles Martorell**[1], **Rubén Calvo**[1], **Adrián Roig**[1], **Alessia Annibale**[2], **and Miguel A. Muñoz**[1]

[1] Departamento de Electromagnetismo y Física de la Materia and Instituto Carlos I de Física Teórica y Computacional, Universidad de Granada, E-18071 Granada, Spain

[2] Department of Mathematics, King's College London, London WC2R 2LS, United Kingdom

E-mail: `carlesma@ugr.es`

October 9, 2025

*Keywords*: Ergodic theory, Spin glasses, Chaotic dynamics, Neural networks. Submitted

to: *J. Stat. Mech.*

## 1. Path–integral formulation

Throughout this section, the microscopic dynamics are governed by an $N$-dimensional Langevin equation with additive noise,

$$\partial_t x_i(t) = -x_i(t) + \phi\left(\sum_{j=1}^{N} W_{ij} x_j(t)\right) + \sqrt{2}\sigma\, \xi_i(t), \tag{1}$$

where $\partial_t$ denotes the time derivative, $\phi(x)$ is a nonlinear gain function (typically $\tanh(x)$), $W_{ij}$ are quenched synaptic weights, and $\xi_i(t)$ is a white-noise term. The connectivity matrix $\mathbf{W}$ is drawn from a Gaussian ensemble with mean $\overline{W_{ij}} = J_0/N$ and variance $\overline{W_{ij}^2} - J_0^2/N^2 = J^2/N$, ensuring finite input per unit as $N \longrightarrow \infty$. Here, $\bar{\cdot}$ denotes averaging over the distribution of matrices, i.e. quenched disorder.

The aim of this appendix is to show how the dynamical mean–field (DMF) formulation arises from a path–integral description. Using the Martin–Siggia–Rose–Janssen–de Dominicis (MSRJD) framework [1, 2], we demonstrate that, in the thermodynamic limit, the system's statistics reduce to those of a single effective neuron. This effective one–neuron system is governed by a stochastic differential equation, the DMF equation. Finally, we show that DMF observables reduce to Gaussian integrals over the effective noise, providing both a rigorous foundation for the DMF equations and a direct link between statistical–physics methods and stochastic dynamical systems.

An introduction to the MSRJD formalism and its applications in disordered systems can be found in [1–6].

### *1.1. From stochastic trajectories to a MSRJD action*

For a fixed (quenched) connectivity matrix $\mathbf{W}$ and an initial condition $\mathbf{x}(0) = \mathbf{x}_0$, each realization of the external white noise $\xi(t)$ generates a unique trajectory $\mathbf{x} : t \mapsto \mathbf{x}(t) \in \mathbb{R}^N$; where bold symbols denote vectors, i.e. $\mathbf{x}(t) = [x_1(t), ..., x_N(t)]^T$. Additionally, a trajectory over time will be denoted by $\underline{\mathbf{x}} = \mathbf{x}(t)_{0\leq t\leq T}$, in the time interval $[0, T]$.

The Martin–Siggia–Rose–Janssen–de Dominicis (MSRJD) construction [1–3], assuming the Itô convention, assigns to each trajectory a weight $\exp(-S[\underline{\mathbf{x}}, \underline{\tilde{\mathbf{x}}}])$ defined by the action

$$S[\underline{\mathbf{x}}, \underline{\tilde{\mathbf{x}}}] = \int_0^T dt \sum_{i=1}^N \Big[\tilde{x}_i(t)\big(\partial_t x_i(t) + x_i(t) - \phi(g\sum_j W_{ij}x_j(t))\big) + \sigma^2\tilde{x}_i^2(t)\Big], \qquad (2)$$

where $\tilde{x}_i(t)$ is an auxiliary response field introduced by the delta constraint enforcing the Langevin dynamics. The quadratic term $\sigma^2\tilde{x}_i^2(t)$ arises from integrating over the Gaussian noise. Thus the functional weight vanishes unless the stochastic dynamics are satisfied.

All statistical properties of the process are encoded in the moment-generating functional (MGF)

$$Z[\underline{j}, \underline{\tilde{j}}] = \int \mathcal{D}\underline{\mathbf{x}}\,\mathcal{D}\underline{\tilde{\mathbf{x}}}\ \exp\Big\{-S[\underline{\mathbf{x}}, \underline{\tilde{\mathbf{x}}}] + \int_0^T dt \sum_i \big(j_i(t)x_i(t) + \tilde{j}_i(t)\tilde{x}_i(t)\big)\Big\},$$

where $\underline{j}$ and $\underline{\tilde{j}}$ are source fields. We assume that the path integral is normalized, such that $Z[0, 0] = 1$. The functional derivatives of $Z$ reproduce the full hierarchy of correlation and response functions; for example

$$\langle x_i(t)\, x_j(s)\rangle = \frac{\delta^2 Z}{\delta j_i(t)\,\delta j_j(s)}\Big|_{j,\tilde{j}=0}.$$

As an important remark, the conjugate source field $\underline{\tilde{j}}$ can be interpreted as an external perturbation to the dynamics. It enters the action as a linear contribution to the dynamical equation and generates the response field $\tilde{x}(t)$. As a consequence, one obtains the identity

$$\langle \tilde{x}_i(t)\, x_j(s)\rangle \;=\; \frac{\delta\langle x_j(s)\rangle}{\delta\tilde{j}_i(t)}\,,$$

Thus, the auxiliary field $\tilde{x}_i(t)$, while introduced as a mathematical device, obtains the physical interpretation of generating linear response function to an external perturbation $\tilde{j}_i(t)$.

### *1.2. Disorder average and collective fields*

Averaging the MGF over the Gaussian ensemble of couplings removes sample-to-sample fluctuations. The resulting disorder-averaged functional, denoted by

$$\overline{Z}[j,\tilde{j}] \;=\; \big\langle Z[j,\tilde{j};W]\big\rangle_W,$$

can be reduced to that of a *single* effective neuron by three standard steps (for the current derivation, see [7]; for additional details, see [4–6]).

(i) *Input currents.* By using the Fourier representation of the Dirac delta function, we introduce the synaptic currents $z_i(t) = g\sum_j W_{ij}x_j(t)$ on the MGF, transforming the action into a linear expression, reproducing the SCS [4, 8] form in terms of $z_i(t)$ and its Fourier conjugate $\tilde{z}_i(t)$. Notably, by means of the synaptic current this establishes a correspondence between our firing-rate system and the original SCS system, meaning that the results of the later are valid in terms of $z_i(t)$ in our system.

(ii) *Hubbard–Stratonovich transformation.* The resulting Gaussian average over $W_{ij}$ yields quadratic terms of the microscopic $z_i(t)$ and $\tilde{z}_i(t)$ fields, which are linearised by introducing collective (order-parameter) fields by means of a Hubbard-Stratonovich transformation. The most relevant order parameters are the (population) mean activity and the two-time autocorrelation,

$$M(t) = \frac{1}{N}\sum_{i=1}^{N} x_i(t), \qquad C(t,s) = \frac{1}{N}\sum_{i=1}^{N} x_i(t)\, x_i(s).$$

The saddle-point selection of these observables is, indeed, the demonstration of the self-averaging property.

(iii) *Saddle point.* In the thermodynamic limit $N \longrightarrow \infty$, the functional integral of the MGF is evaluated by the saddle–point (steepest–descent) method: the dominant contribution arises from the configuration of the macroscopic fields that extremizes the action, while fluctuations are suppressed as $1/N$. These extremal configurations define the saddle–point solutions. In this limit, the disorder–averaged MGF factorizes, meaning that correlations between different units vanish and the network becomes equivalent to $N$ uncoupled copies of a single effective generating functional,

$$\overline{Z}[j,\tilde{j}] \xrightarrow{N\to\infty} Z_{\text{eff}}[j,\tilde{j}]. \tag{3}$$

Accordingly, in the thermodynamic limit, the system's statistics are identical to those of an effective one-unit system, where the MGF is given by

$$Z_{\text{eff}}(\underline{j},\underline{\tilde{j}}) = \int \mathcal{D}[\underline{x},\underline{\tilde{x}},\underline{z},\underline{\tilde{z}}]\exp\left(-S_{\text{eff}}[\underline{x},\underline{\tilde{x}},\underline{z},\underline{\tilde{z}}] + \int dt\; x(t)j(t) + \tilde{x}(t)\tilde{j}(t)\right) \tag{4}$$

The action is described as:

$$S_{\text{eff}}[\underline{x}, \underline{\tilde{x}}, \underline{z}, \underline{\tilde{z}}] = \int_0^T dt\ \tilde{x}(t)\ \big(\partial_t x(t) + x(t) - \phi(z(t)) - \sigma^2 \tilde{x}(t)\big) \tag{5}$$

$$+ \int_0^T dt\ \tilde{z}(t)\ \big(z(t) - gJ_0 M(t)\big) \tag{6}$$

$$- \frac{g^2 J^2}{2} \iint_0^T dt\, ds\ \tilde{z}(t)\, C(t,s)\, \tilde{z}(s), \tag{7}$$

where the three contributions have distinct roles: (i) Eq. (5) is the delta constraint that enforces the Langevin dynamics of the effective neuron, (ii) Eq. (6) introduces the constraint on the effective input current, and (iii) Eq. (7) generates correlations induced by the quenched disorder.

The last term, Eq. (7), can be recast as the contribution of an effective Gaussian noise $\eta(t)$ with zero mean and covariance

$$\langle \eta(t)\eta(s) \rangle = C(t,s).$$

Integrating out the auxiliary field $\tilde{z}$ reduces the action to the pair of fields $(x, \tilde{x})$ subject to this effective stochastic input:

$$S_{\text{eff}}[\underline{x}, \underline{\tilde{x}}, \underline{\eta}] = \int_0^T dt\ \tilde{x}(t)\ \Big[\partial_t x(t) + x(t) - \phi\big(gJ_0 M(t) + gJ\eta(t)\big) - \sigma^2\, \tilde{x}(t)\Big]. \tag{8}$$

Accordingly, the generating functional of the effective single-neuron system takes the form

$$Z_{\text{eff}}[\underline{j}, \underline{\tilde{j}}] = \int \mathcal{D}[\underline{x}, \underline{\tilde{x}}, \underline{\eta}]\, P[\underline{\eta}]\ \exp\bigg(-S_{\text{eff}}[\underline{x}, \underline{\tilde{x}}, \underline{\eta}] + \int_0^T dt\ [x(t)j(t) + \tilde{x}(t)\tilde{j}(t)]\bigg), \tag{9}$$

where $P[\underline{\eta}]$ denotes the Gaussian path measure of the noise $\eta(t)$.

### *1.3. Emergent Dynamical Mean Field*

The effective MGF described in Eq.(9) yields the effective stochastic equation

$$\partial_t x(t) = -x(t) + \phi\left(gJ_0 M(t) + gJ\eta(t)\right) + \sqrt{2}\sigma\, \xi(t), \tag{10}$$

where $\xi(t)$ is the original white noise and $\eta(t)$ is a *self–generated Gaussian process* with

$$\langle \eta(t) \rangle = 0, \qquad \langle \eta(t)\eta(s) \rangle = C(t,s). \tag{11}$$

Equations (10)–(11) are the DMF closure: the $N$–dimensional network reduces to a single non-linear stochastic process driven by colored noise whose statistics are self–consistently determined.

### *1.4. From path integrals to stochastic dynamics*

The effective moment–generating functional (9) is exactly equivalent to the DMF stochastic equation (10). Thus, the path–integral description can be reformulated as a stochastic differential equation driven by the Gaussian process $\eta(t)$. This establishes a bridge between statistical–physics methods and stochastic dynamical systems.

To make this explicit, we extend the MSRJD construction to a general stochastic differential equation of the form

$$\partial_t x(t) = f\big(x(t), \eta(t)\big) + \sqrt{2}\,\sigma\,\xi(t), \tag{12}$$

where $\xi(t)$ is Gaussian white noise and $\eta(t)$ an auxiliary stochastic process. Such dynamics are represented by a generating functional over $x(t)$ and its response field $\tilde{x}(t)$, with an action identical to that introduced previously, plus the linear coupling

$$\int_0^T dt\,\tilde{x}(t)\,f\big(x(t), \eta(t)\big).$$

Since $\eta(t)$ enters only through this linear term, averaging over its distribution is mathematically well defined. Applying this reasoning to the DMF equation (10) yields precisely the effective MGF in Eq. (9), thereby justifying the derivation. Consequently, the stochastic averages underlying the DMF closure are fully consistent with the MSRJD framework and equivalent to those of the effective stochastic dynamics in Eqs. (10)–(11).

### *1.5. Consistency of noise averaging in the DMF formalism*

In the DMF formulation, averages are defined over the path distribution of the effective system. In this subsection we show that, instead of relying on the full path–integral formalism, these averages can be equivalently expressed as integrals over the probability distribution of the effective noise $\eta(t)$. Since $\eta(t)$ is Gaussian, the computation reduces to Gaussian integrals, providing a simpler and consistent justification of the DMF averages.

Let $\mathcal{O}(\underline{x}, \underline{\tilde{x}})$ be an observable. Its expectation under the effective dynamics determined by Eq. (9) is defined as

$$\langle \mathcal{O}(\underline{x}, \underline{\tilde{x}}, \underline{\eta}) \rangle = \int \mathcal{D}[\underline{x}, \underline{\tilde{x}}, \underline{\eta}]\, P(\underline{\eta})\, \mathcal{O}(\underline{x}, \underline{\tilde{x}}, \underline{\eta})\, e^{-S_{\mathrm{eff}}[\underline{x}, \underline{\tilde{x}}, \underline{\eta}]}. \tag{13}$$

As an example, consider the average of the non-linear input signal, defined by

$$\Big\langle \phi(gJ_0M(t) + gJ\eta(t)) \Big\rangle, \tag{14}$$

which requires averaging over $\eta(t)$. Since $\eta(t)$ is a Gaussian process with zero mean and covariance $C(t,s)$, its joint probability distribution can be formally written as

$$P(\underline{\eta}) = \prod_{t',t''} P(\eta(t'), \eta(t'')) = \prod_{t',t''} \frac{1}{2\pi\sqrt{\det \Sigma(t',t'')}} \exp\left[-\tfrac{1}{2}\,\tilde{\eta}^T_{t',t''}\,\Sigma(t',t'')^{-1}\,\tilde{\eta}_{t',t''}\right], \tag{15}$$

where $\tilde{\eta}^T_{t',t''} = [\eta(t'), \eta(t'')]$ and the covariance matrix is

$$\Sigma(t', t'') = \begin{bmatrix} C(t', t') & C(t', t'') \\ C(t', t'') & C(t'', t'') \end{bmatrix}. \tag{16}$$

The path measure therefore factorizes into two-time coupled terms –or, equivalently, bivariate Gaussian distributions. To compute the nonlinear average at a fixed time $t$, we select the pair $(t', t'') = (t, s)$. Since the nonlinear observable depends only on $\eta(t)$, all factors with $s \neq t$ integrate to unity by normalization. Thus only the marginal distribution at time $t$ contributes, which is Gaussian with variance $C(t, t)$. Consequently, one obtains

$$\Big\langle \phi(gJ_0M(t) + gJ\eta(t)) \Big\rangle = \int_{-\infty}^{+\infty} Du\, \phi\Big(gJ_0M(t) + gJ\sqrt{C(t,t)}\, u\Big), \tag{17}$$

where $Du = e^{-u^2/2}du/\sqrt{2\pi}$.

A similar reasoning applies to two–time observables. For instance, the nonlinear autocorrelation, the $\Xi$-function,

$$\Big\langle \phi\big(gJ_0M(t) + gJ\eta(t)\big)\, \phi\big(gJ_0M(s) + gJ\eta(s)\big) \Big\rangle, \tag{18}$$

reduces to an integral with respect to the bivariate Gaussian law, $P(\eta(t), \eta(s))$, defined by $\Sigma(t, s)$ (the details of this derivation are described in the Appendix).

Therefore, averages in the DMF formalism reduce systematically to Gaussian integrals over $\eta(t)$ or $(\eta(t), \eta(s))$. This establishes that stochastic averages at the SDE level are mathematically well defined, and ensures that the DMF closure reproduces the self–consistent equations for the mean activity and autocorrelation [see Appendix].

## References


[1] Martin P C, Siggia E D and Rose H A 1973 *Physical Review A* **8** 423–437 ISSN 0556-2791 URL `https://link.aps.org/doi/10.1103/PhysRevA.8.423`

[2] De Dominicis C and Peliti L 1978 *Physical Review B* **18** 353–376 ISSN 0163-1829 URL `https://link.aps.org/doi/10.1103/PhysRevB.18.353`

[3] Hertz J A, Roudi Y and Sollich P 2017 *Journal of Physics A: Mathematical and Theoretical* **50** 033001 ISSN 1751-8113, 1751-8121 URL `https://iopscience.iop.org/article/10.1088/1751-8121/50/3/033001`

[4] Helias M and Dahmen D 2020 *Statistical Field Theory for Neural Networks* (*Lecture Notes in Physics* vol 970) (Cham: Springer International Publishing) ISBN 978-3-030-46443-1 978-3-030-46444-8 URL `http://link.springer.com/10.1007/978-3-030-46444-8`

[5] Zou W and Huang H 2024 *SciPost Physics Lecture Notes* 79 ISSN 2590-1990 arXiv:2305.08459 [cond-mat, q-bio] URL `http://arxiv.org/abs/2305.08459`

[6] Galla T 2024 Generating-functional analysis of random Lotka-Volterra systems: A step-by-step guide arXiv:2405.14289 [cond-mat, q-bio] URL `http://arxiv.org/abs/2405.14289`

[7] Martorell C, Calvo R, Annibale A and Muñoz M A 2024 *Chaos, Solitons & Fractals* **182** 114809 ISSN 09600779 URL `https://linkinghub.elsevier.com/retrieve/pii/S0960077924003618`

[8] Crisanti A and Sompolinsky H 2018 *Physical Review E* **98** 062120 ISSN 2470-0045, 2470-0053 arXiv:1809.06042 [cond-mat] URL `http://arxiv.org/abs/1809.06042`
